# Supplementary material for: Robust surface states and coherence phenomena in magnetically alloyed SmB6
Source: arXiv:1907.07074 ancillary file (2021-05-25)
Supplement: Supplementary file 1 [file SmB6_SI_0119.pdf]

*Supplementary Information for*

# Robust coherence phenomena and surface states in magnetically alloyed $SmB_6$


Lin Miao,[1] Chul-Hee Min,[2] Yishuai Xu,[3] Zengle Huang,[4] Erica C. Kotta,[3] Rourav Basak,[3] M. S. Song,[5] B. Y. Kang,[5] B. K. Cho,[5] K. Kißner,[2] Friedrich Reinert,[2] Turgut Yilmaz,[6] Elio Vescovo,[6] Yi-De Chuang,[7] Weida Wu,[4] Jonathan D. Denlinger,[7] and L. Andrew Wray[3]

1. School of Physics, Southeast University, Nanjing, 211189, China
2. Experimentelle Physik VII and Würzburg-Dresden Cluster of Excellence ct.qmat, Universität Würzburg, Am Hubland, D-97074 Würzburg, Germany
3. Department of Physics, New York University, New York, New York 10003, USA
4. Rutgers Department of Physics and Astronomy, Rutgers University, Piscataway New Jersey 08854, USA
5. School of Materials Science and Engineering, Gwangju Institute of Science and Technology (GIST)
6. National Synchrotron Light Source II, Brookhaven National Lab, Upton, New York 11973, USA
7. Advanced Light Source, Lawrence Berkeley National Laboratory, Berkeley, CA 94720, USA

**Corresponding author：**

L. Andrew Wray    Email: lawray@nyu.edu


**This PDF file includes:**

Supplementary text

Figures S1 to S11

SI References

**Table of Contents**

Supplementary Note **1**: Growth of $Sm_{1-x}M_xB_6$ samples

Supplementary Note **2**: Homogeneity of the alloyed samples and cleaved surfaces

Supplementary Note **3**: The influence of aging on ARPES measurements

Supplementary Note **4**: The resistivity and susceptibility measurements

Supplementary Note **5**: Topological significance of the $\bar{X}$ -point pocket

Supplementary Note **6**: Dopant valence states

Supplementary Note **7**: Fitting local moments

Supplementary Note **8**: Mapping topological 2D states

Supplementary Note **9**: Anderson localization, and the persistence of surface states without a surface conductivity plateau.

**Supplementary Note 1: Growth of $Sm_{1-x}M_xB_6$ samples**

Single crystals of $Sm_{1-x}M_xB_6$ (M = Eu, Ce) were prepared by the alumina flux method. The stoichiometric mixture of the rare-earth metal (99.9%, Alfa Aesar) and boron pieces (99.9%, RND Korea) was placed in an alumina crucible (99.8%, Samhwa Ceramic Company) with Al (99.999%, RND Korea) as a metal-flux at a mass ratio of $Sm_{1-x}M_xB_6$ : Al = 1:50. The mixture was heated in a vertical tube furnace with a $MoSi_2$ heating element. The heating profile was started by heating to 300°C for one hour to flush the oxygen from the system in a flowing high-purity argon atmosphere (99.999%) at a rate of 0.55 l/min. After dehydration, the mixture was then heated to T=1600°C at a rate of 325°C/h and maintained at 1600°C for 4 hours. The crystals grew in the cooling step that followed, from T=1600°C to T=650°C at a rate of 4.8°C/h, and the furnace was then shut off because it was below the aluminum melting point. The single crystals were separated from the Al flux using NaOH solution. The crystal structure of samples was characterized using powder X-ray diffraction (XRD; Rigaku D/MAX-2500 with Cu target) at room temperature.

**Supplementary Note 2: Homogeneity of the alloyed samples and cleaved surfaces**

In the main text, $Sm_{0.8}Eu_{0.2}B_6$ and $Sm_{0.7}Ce_{0.3}B_6$ are investigated by ARPES to show the robust in-gap surface state. Care is required to ensure that these measurements are representative of a uniform alloy, and do not merely derive from Sm-rich regions. Supplementary analyses show that such a determination can be made self-consistently with a range of experimental techniques, including:

1. X-ray diffraction (XRD) spectrum confirms a single-phase growth, with no recognized impurities (Fig. S1).
2. Scanning tunneling microscopy (STM) topography maps show flat surfaces and uniform doping-associated mosaicity in surveys of the cleaved sample surfaces (Fig. S2-3). Dopant atom density (observed for $Sm_{0.8}Eu_{0.2}B_6$), and associated surface texture (for both samples) were consistent with the nominal concentration of Eu/Ce atoms.
3. Ultraviolet X-ray photoemission spectroscopy (UPS) on the prominent Eu multiplet features reveal a uniform environment for Eu atoms in $Sm_{0.8}Eu_{0.2}B_6$ that differs significantly from $EuB_6$ (Fig. S4).
4. Magnetic susceptibility measurements show a sharp magnetic transition within ±1K in $Sm_{0.8}Eu_{0.2}B_6$, implying a uniform Eu concentration (see Fig. 3(b) of the main text). The Néel temperature of $Sm_{1-x}Eu_xB_6$ grows rapidly near x=0.2 and has been attributed as $T_N$=0 at x=0.15 and $T_N$=12K at x=0.25 [1]. A naïve linear extrapolation between these points yields an upper bound of ±0.01 in the regional variability of x within our sample. Attributing a more natural phase contour, such as that proposed in Ref. [1] as a guide to the eye, can significantly reduce the upper bound.
5. ARPES measurements of both samples show that no Fermi level feature is present at the extrapolated Fermi momentum of the bulk Sm 5*d* band. Together with the sharp

lineshape of the 5d band beneath the Fermi level, this observation indicates that the Kondo gap was uniformly robust beneath the ~50×100 $\mu m^2$ beam spot. This characterization is reviewed as a function of time in Fig. S5.

In spite of the overall homogeneity, alloying will nonetheless introduce significant disorder, presenting a challenging environment for Kondo physics. Some Kondo systems have been noted to be very sensitive to disorder [2-4], and disorder that creates voids in dense Kondo lattices is known to destabilize the Kondo lattice via the creation of "Kondo holes" [5-6]. The persistence of topological Kondo(-like) physics within the alloyed environment we have imaged is exceptional, and recent theory suggests that a robust gap may be intrinsic to the physics of mixed-valent insulators [7]. In this context, it is noteworthy that the mixed-valent nature of Sm provides a degree of freedom within the same symmetry sector as a Kondo hole ($Sm^{2+}$ is pseudospin 0, like a Kondo hole). This enables a reconfiguration of the Kondo lattice that may effectively screen Kondo holes. A very recent study on non-stoichiomentric $SmB_6$ has also found a robust gap structure in the presence of even greater disorder (as $Sm_{0.6}B_6$) [8].

**Supplementary Note 3: The influence of aging on ARPES measurements**

Our previous investigations have revealed significant valence state changes at the surface of cleaved $SmB_6$ surfaces within ultrahigh vacuum (UHV), on the time scale of hours to days [9,10], which appear to involve a conversion of surface samarium to $Sm^{3+}$ atomic multiplet states [9]. Similar changes in high energy multiplet-derived features are seen in ARPES spectra (see $Ce_{0.3}Sm_{0.7}B_6$ data in Fig. S5 (a-b)) but have a remarkably negligible impact on Kondo-associated features at the Fermi level (see Fig. S5 (c-e)). As samples age, a broad feature centered at E~-0.7eV, loses spectral weight, and a sharper feature at higher binding energy (E~-0.8eV) grows more subtly in intensity (Fig. S5 (a-b) and (e)). The ~-0.7 eV feature has been identified with excess surface $Sm^{2+}$ in earlier studies [11], making these changes consistent with the expectation of an oxidizing trend. These trends are consistent with a previous study of $Eu_{0.15}Sm_{0.85}B_6$, in which aging was found to weaken the E~-0.7eV feature but have little impact on angle-integrated photoemission within ~20meV to the Fermi level [12].

**Supplementary Note 4: The resistivity and susceptibility measurements**

Magnetic susceptibility of all samples was measured using a Quantum Design PPMS vibrating sample magnetometer (VSM) with a magnetic field of 500 Oe applied along the <001> direction of $SmB_6$. The mass of samples used for susceptibility was studies 11.5mg (5% Eu), 6.5mg (10% Eu), 9.4mg (20% Eu), 2.3mg (1% Ce), 12.3mg (3% Ce), 6.0mg (10% Ce), 5.0mg (30% Ce). Transport measurements made use of larger slightly polished near-cubic samples (1.2 mm - 1.5 mm per edge), and the current was

applied along the <100> direction. These data are presented in units of 3D bulk resistivity (Ω-m), and are expected to be bulk-dominated for all doped samples due to the combination of cubic sample geometry, reduced resistivity relative to the undoped sample, and enhanced localization of surface electrons (see Supplementary Note 9). Nonetheless, the use of bulk resistivity units should not be taken to rule out some contribution from 2D surface transport.

**Supplementary Note 5: Topological significance of the $\overline{X}$ -point pocket**

The surface $\overline{X}$ -point Fermi pocket (and $\overline{X}$ - $\overline{M}$ momentum trajectory) is selected for the topological analysis in this investigation because an $\overline{X}$ -point pocket is the most reliably visible feature in ARPES studies of $SmB_6$, and because this feature has been confirmed to be singly degenerate by spin-resolved (spin-ARPES) investigations [13,14]. When taken at face value, the ARPES and spin-ARPES measurements of the $\overline{X}$ -point pocket directly imply a non-trivial bulk topology. A recent study incorporating spin-ARPES has found that the bulk X-point inversion underlying the surface $\overline{X}$ -point Fermi pocket gives rise to a similar topological surface state on the (111) surface as well [15]. This section will briefly review the topological scenario presented by $SmB_6$, the potential role of surface band bending, and alternative interpretations of the band structure.

The bulk band structure of $SmB_6$ features a 5d/4f band inversion at the bulk X-point [11,16]. In a single-particle-based picture, this scenario combined with the crystal structure guarantees that all 5d/4f hybridization gaps will be 'topological gaps' [16,17], with associated symmetry inversions labeled by minus signs in Fig. S6(a, center). This is typically expected to result in the appearance of singly degenerate surface state pockets surrounding the surface $\overline{X}$ and $\overline{\Gamma}$ points (see Fig. S6(a, bottom) diagram), and a non-trivial topology can be noted by counting an odd number of surface state crossings along any path between the surface $\overline{X}$ - and $\overline{M}$ -points, or the $\overline{\Gamma}$ - and $\overline{M}$ -points [18].

All $SmB_6$ ARPES measurements that we are aware of agree on there being a single $\overline{X}$ -point pocket, making the $\overline{X}$ - $\overline{M}$ axis relatively easy to focus on for

identifying nontrivial topology. By contrast, features surrounding the $\overline{\Gamma}$ -point tend to be weaker and are often missed entirely, likely due to matrix element effects such as the orbital angular momentum barrier for small-angle photoemission [19], and are not as consistently observed. Moreover, though many measurements show zero or one Fermi pockets surrounding the $\overline{\Gamma}$ -point, up to 5 distinct surface states are suspected to exist, including two Umklapp-scattered rings [11,13-20], a pair of Rashba-split states [20], and an additional state required by topology. The weakness of these features tends to be prohibitive for spin-ARPES, rendering a definitive analysis even more challenging. This paper does not seek to evaluate $\overline{\Gamma}$ -point band structure for these reasons, and because understanding the $\overline{X}$ -point band structure is sufficient to establish a topologically nontrivial scenario. Though we do not attempt a full map of the topological indices, further measurements at the remaining 2D high symmetry points are presented in Supplementary Note 8, and are consistent with expectations for a strong TI state.

In spite of the case presented above, there remain alternative proposals for interpreting the $\overline{X}$ -point topology. A recent paper has shown that with improved measurement resolution it is possible to resolve details of band structure surrounding the $\overline{X}$ -point that do depend on the surface chemistry, and can be interpreted as evidence of band bending [20]. A possible trivial surface band structure proposed in Ref. [20] is outlined in Fig. S6 (b, bottom), with the $\overline{\Gamma}$ -point ring attributed as a trivial artifact of Umklapp scattering, and the $\overline{X}$ -point Fermi pocket structure attributed as a doubly degenerate 2D electron gas derived from band bending. While this analysis is intriguing, the existence of a spin-degenerate 2D electron gas is contradicted by spin-ARPES. Moreover, the proposed semiconductor-like band bending paradigm is not questionable for Kondo systems, and STM measurements of electronic density of states curves at chemically different surface terminations of $SmB_6$ look extremely similar within 50 meV of the Fermi level, where the Kondo coherent band structure is found (see Fig. 3 of Ref. [21]). An extensive recent STM investigation of $SmB_6$ polar surfaces suggests no variation in the basic topological scenario presented at the $\overline{X}$ -point, and extremely little band structure sensitivity for the [2x1]-reconstructed surfaces predominantly found in our topographical maps [22].

Recent literature has further noted that the feature attributed as an Umklapp artifact does not have the same group velocity (slope) as the band it is believed to duplicate, suggesting that there is insufficient evidence to neglect this feature when evaluating surface topology [15]. Together with the consistent indication from spin-ARPES that the X-point pocket is singly degenerate, this observation can render the same surface band structure compatible with a strong TI scenario (see supplementary note 9 of Ref. [15]).

**Supplementary Note 6: Dopant valence states**

The valence state of dopant Ce is identified by *N*-edge (4*d*-4*f*) X-ray absorption spectroscopy (XAS) on $Sm_{0.7}Ce_{0.3}B_6$ (Fig. S7(a)). The N-edge XAS of Sm is seen an energy window from 130eV to 150eV, and features weight from both $Sm^{2+}$ and $Sm^{3+}$, with a time-dependent drift towards $Sm^{3+}$ [23]. The N-edge XAS spectrum of Ce features sharply resolved fine structure at hv<115 eV that closely matches atomic multiplet simulation for the $4f^1$ confirguration. The one-to-one fitting of the peaks between the $4f^1$ simulation and the XAS curves indicates a relatively pure $Ce^{3+}$ valence state of the dopant Ce in $Sm_{0.7}Ce_{0.3}B_6$.

Europium is known to be divalent in $EuB_6$. Here, the divalent nature of dopant Eu is distinguished by a valence photoemisson measurement on $Sm_{0.8}Eu_{0.2}B_6$. The strong features centered at $E_B$~1.5 eV binding energy are $Eu^{2+}$ multiplets, and match the presentation in $EuB_6$ [24]. Moreover, by using the same excitation photon energy of $h\upsilon$=70eV, we find that EuO and $Sm_{0.8}Eu_{0.2}B_6$ share the same pronounced peak at $E_B$~5eV and a shallow broad peak around $E_B$~9eV [25]. These correspondences strongly suggest a 2+ valence state, but do not rule out the possibility of some fractional $Eu^{3+}$, as $Eu^{3+}$ is also associated with a ~9 eV photoemission multiplet feature. Both ARPES and XAS results show mixed signals from Sm and dopants, excluding the possibility of phase separation within the beam-spot.

Atomic multiplet calculations for $Ce^{3+}$ were performed for the N-edge ($4d^{10}4f^1 \rightarrow 4d^9 ff^2$ X-ray absorption) in the dipole approximation. Hartree-Fock parameters were obtained from the Cowan code [26], and full diagonalization of the multiplet Hamiltonian was performed using LAPACK drivers [27]. Hartree-Fock parameters for 4*f* multipole interactions were renormalized by a factor of $\beta$=0.8, Core-valence multipole interactions renormalized by $\beta_C$=0.7. The core hole inverse lifetime is $\Gamma$=0.3 eV at $h\upsilon$<117eV, $\Gamma$=7 eV at 117 eV<$h\upsilon$<120 eV, and 9 eV at $h\upsilon$>120 eV.

**Supplementary Note 7: Fitting local moments**

The effective moment of the magnetically alloyed $SmB_6$ is extracted by fitting the

inverse susceptibility with Curie-Weiss law of the paramagnetic phase, which can be described as:

$$\chi=\chi_0 + N_A\mu_0 \mu_J^2 / (3k_B(T-\Delta)) \quad (1)$$

The $N_A$ is the Avogadro constant, $k_B$ is Boltzmann's constant, $\mu_0$ is the permeability of free space, and T is the temperature in Kelvin. The parameter Δ is the Curie-Weiss temperature. The $\chi_0$ offset is a temperature-independent background, and it is paramagnetic with a value of ~$10^{-5}$ emu in our system. Fitting at T>200K (see Fig. S8) yields effective moments of 5.4$\mu_B$ (1%), 5.15$\mu_B$ (3%), 4.2$\mu_B$ (10%) and 3.15$\mu_B$ (30%) for the Ce-alloyed $SmB_6$, and 4.1$\mu_B$ (5%), 7.1$\mu_B$ (10%) and 6.1$\mu_B$ (20%) for the Eu-alloyed $SmB_6$. The fitted Δ values are negative, with amplitudes of 382K (1% Ce), 374K (3% Ce), 213K (10% Ce), 56K (30% Ce), 222K (5% Eu), 321K (10% Eu) and 162K (20% Eu).

Heavy Fermion compounds are known to show large negative Curie-Weiss temperatures, and Curie-Weiss fits can yield sensible local moment values in spite of this [28-30]. The Curie-Weiss temperatures fitted here for more lightly doped samples are nonetheless surprisingly large, and we note that imposing a cap of Δ =-200K on the Curie-Weiss temperature and forcing an intercept at T=250K with the fit curve would reduce the lightly doped (1% Ce) end point susceptibility by roughly 16%, to 4.55$\mu_B$.

## Supplementary Note 8: Mapping topological 2D states

**Two-dimensionality:** To verify that the in-gap states we observed in highly magnetically alloyed $SmB_6$, their dimensionality was checked by measuring the surface-normal $k_z$-dependence of ARPES spectra in $Sm_{0.7}Ce_{0.3}B_6$ samples. The two-dimensionality of states at the Fermi level in $Sm_{0.8}Eu_{0.2}B_6$ is less in question, as the sample is bulk-insulating. At low temperature (T=20K), the in-gap states of $Sm_{0.7}Ce_{0.3}B_6$ are non-dispersive along the $k_z$ direction, which clearly indicates two dimensional character (Fig. S10 (b)). One can also see the same non-dispersive surface state in the next Brillouin zone at $k_x$~-1.3$Å^{-1}$. By comparison, the 5*d* bands beneath the Fermi level show an ovoid $k_x$-$k_z$-plane contour (Fig. S10 (c)) that matches their appearance in our map of the $k_x$-$k_y$ plane, as expected from the dimensionality of the sample.

We also performed high-temperature (T=200K) $k_z$-dependence experiment to confirm that the bands crossing the Fermi level are no longer surface states. The $k_x$-$k_z$ map (Fig. S10 (e)) confirms the ovoid contour expected for a three-dimensional band.

This confirms the bulk origin of these states, and rules out the possibility that the spectral features crossing the Fermi level at high temperature are shaped by surface resonance.

**Other required bands:** As discussed in Supplementary Note 5 and the main text, at least one surface state is topologically required to surround the $\overline{\Gamma}$ -point in the attributed strong TI scenario, but we have not focused on these states due to their much weaker spectral weight and possible surface-dependence. At the incident photon energy of 70 eV, surface states at the $\overline{\Gamma}$ -point are not visible for both Eu- and Ce-alloyed $SmB_6$ samples. However, probing incident energy dependence in other Brillouin zones reveals a two-dimensional spectral feature with Fermi momentum $k_x$~-0.2 $Å^{-1}$ that matches expectations for a $\overline{\Gamma}$ -point surface state (red arrows in Fig. S11(e)).

Though it is reassuring to identify a candidate for this feature, the spectral clarity is insufficient for a confident determination of in-plane dispersion (see Fig. S11(a-d)). The signal to background ratio is quite poor, and tilted (seemingly dispersive) striations seen most easily at $k_X>0$ in Fig. S11(e) are associated with slight non-uniformities in the detector. A measurement in a higher Brillouin zone along the $k_Z$-axis (Fig. S11(c-d)) also reveals enhanced intensity near the $\overline{\Gamma}$ -point, but one should note that these data intersect the N-edge resonance of samarium, which may create a spurious background from *f*-orbital multiplet excitation features.

For the sake of completeness in characterizing the topology, it is also noteworthy that no candidate surface state is observed in proximity to the $\overline{M}$ -point, seen at $k_x$~-0.76 $Å^{-1}$ in Fig. S10(b). This is in keeping with expectations for the topology, and with predictions from band structure models.

**Coherence and the bulk band gap:** At high temperature, decoherence of the 4*f* states puts a large and mostly momentum-invariant density of states at the Fermi level, rendering the topological bulk band gap ill defined. Energy dispersion curves in Fig. S12 show the loss of this spectral intensity at the Fermi level as temperature is lowered, which follows the same trend as similar data for the undoped compound [31] and is consistent with the schematic in Fig. 4(c) of the main text.

## Supplementary Note 9: Anderson localization, and the persistence of surface states without a surface conductivity plateau.

As introduced in the main text, papers reporting transport measurements on magnetically doped samples have noted that the low temperature conductivity plateau is lost with <1% magnetic doping, and proposed that this may indicate the loss of topological surface states. Our measurements show that the surface states persist in a nearly unchanged form well beyond the point at which the surface transport signature is lost. The phenomenon of Anderson localization provides a likely context for self-consistent interpretation of the transport and ARPES data.

At a TI surface, the introduction of magnetic dopants (ordered or disordered) is theoretically associated with the loss of weak anti-localization [33,34], meaning that Anderson localization can occur. Anderson localization is a significant phenomenon in 2D systems, and *has the direct consequence that surface conductivity is lost while the 2D surface state bands themselves remain as spectral features and are ungapped*. Strong bulk conduction channels make it difficult to study surface conductivity in TIs other than $SmB_6$, but the existing experimental [35] and numerical modeling [36] examples are consistent with the interpretation that weak anti-localization is easily lost upon magnetic doping, while surface states themselves are more robust.

One must be cautious in extrapolating from theory, as Anderson localization is expected to lose relevance when the length scale of localization is greater than the inelastic mean free path of quasiparticles (i.e. it is not equivalent to many-body localization!). Moreover, Anderson localization is far from the only complicating factor that could reduce long-range electronic mobility at the polar and reconstructed surface of $SmB_6$ alloys. However, our data show that the surface state in alloyed samples is indeed greatly broadened in momentum, suggesting a short length scale for elastic scattering from disorder. The peak width at half maximum of the X-point surface state is roughly ~0.13 $Å^{-1}$ for $Sm_{0.8}Eu_{0.2}B_6$ (and broader for $Sm_{0.7}Ce_{0.3}B_6$) suggesting a mean free path of ~15Å (=2/0.13 $Å^{-1}$) that appears consistent with the length scale of spatial fluctuations seen in our STM data from non-reconstructed surface regions (see Fig. S2(g)).

Lastly, we note that there is no obvious alternative physical mechanism for <~1% magnetic doping inducing the loss of surface states. The basic topological scenario is unchanged in these lightly doped samples, as the material remains an insulator at low temperature, and the topological symmetry inversion that induces surfaces states has a >1eV energy scale associated with the Sm 5*d* band dispersion. Magnetic disorder may induce a gap-like feature at the surface state Dirac point, but the X-point surface state Dirac point is not found within the Kondo gap, and even in the heavily Eu-alloyed magnetic regime, the Néel temperature is sufficiently low ($T_N$<~10K) that one would not expect an associated Zeeman field to greatly impact these bands at the Fermi surface.

**Figure S1**

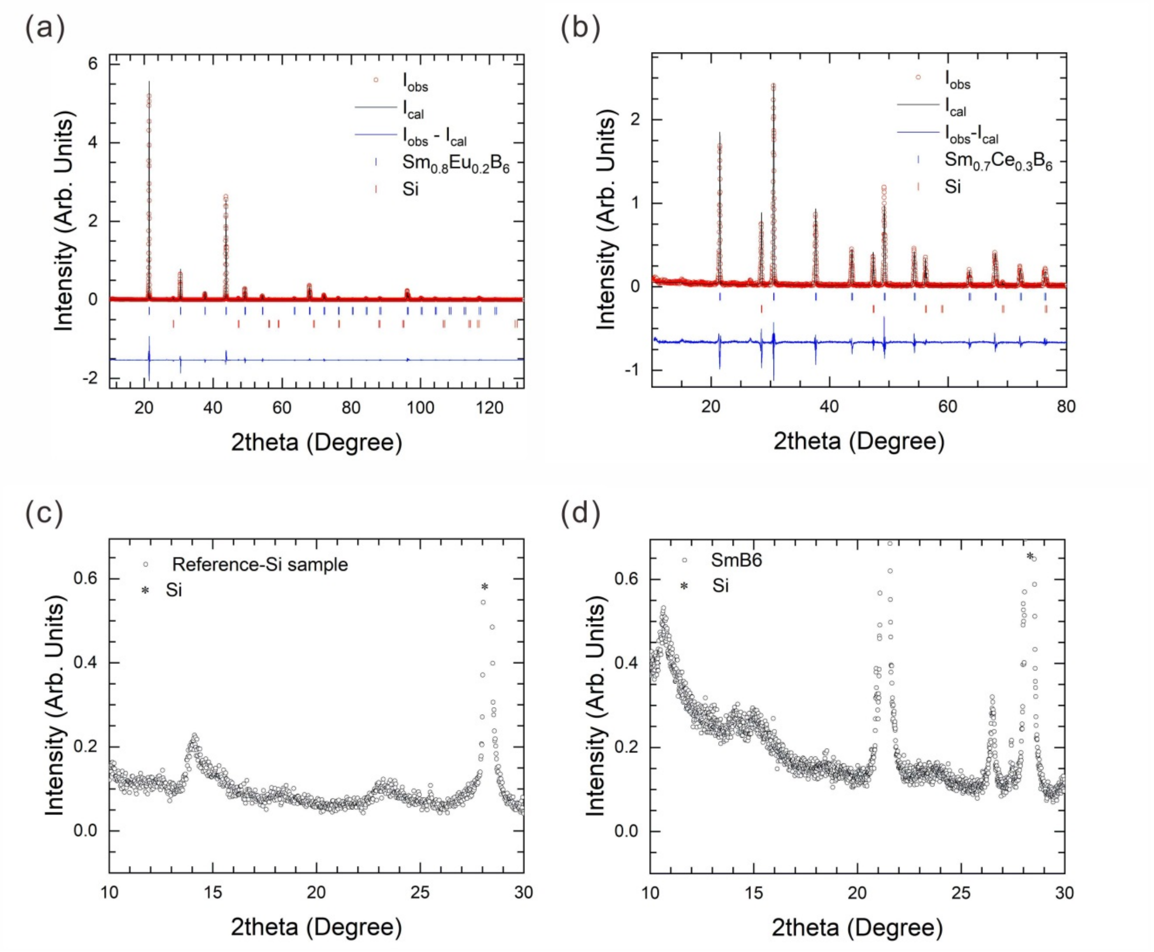


**Fig. S1:** X-ray diffraction spectra of (a) $Sm_{0.8}Eu_{0.2}B_6$ and (b) $Sm_{0.7}Ce_{0.3}B_6$. The spectra are fitted with lattice constants of (a) a=4.1398 Å and (b) 4.13608 Å, and show no evidence of an impurity phase. Very small anomalous features are observable at small angles (especially for $Sm_{0.7}Ce_{0.3}B_6$), and superficially resemble a period-doubling reconstruction (2θ=11°, 15°, 24°, and 27° degrees matching [0.5 0 0], [0.5 0.5 0], [1 0.5 0] and [1 0.5 0.5]). These are attributed as artifacts associated with a contemporary instrumentation maintenance issue. Long-integration spectra from (c) silicon and (d) undoped-$SmB_6$ reference samples show the same phenomenon. Anomalous doubles of the smallest angle Si diffraction features (28° and 47°) are visible at 14° and 23°, respectively.

**Figure S2**

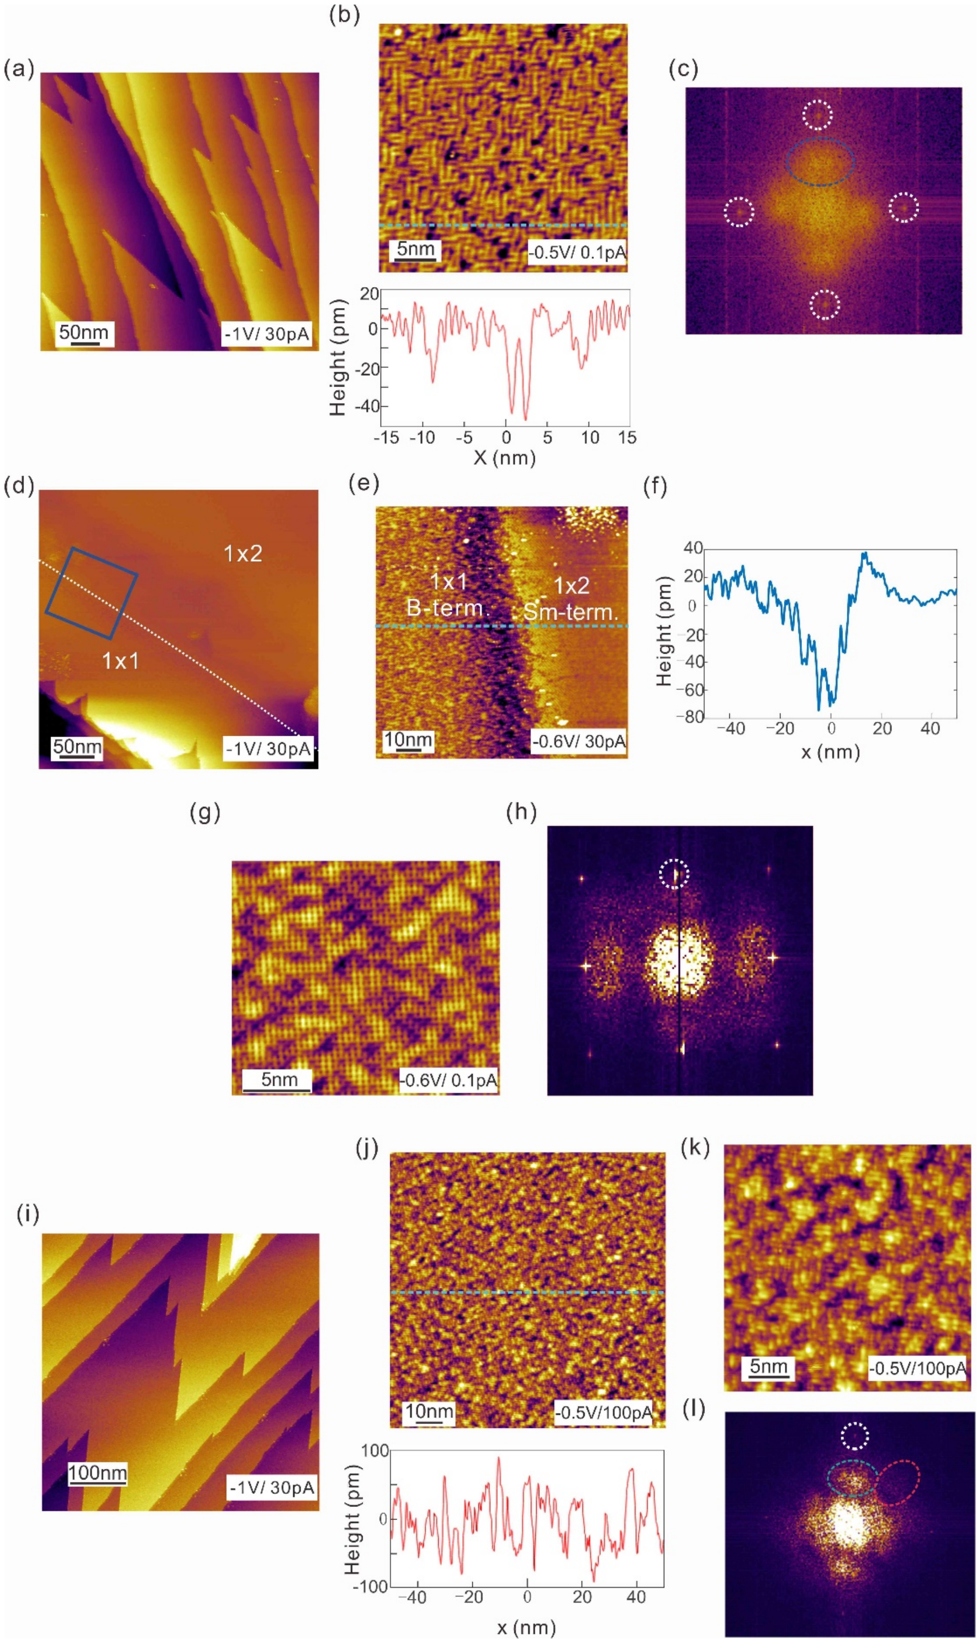
(a)
50nm
-1V/ 30pA
(b)
5nm
-0.5V/ 0.1pA
Height (pm)
X (nm)
(c)
(d)
1x2
1x1
50nm
-1V/ 30pA
(e)
1x1
B-term.
1x2
Sm-term.
10nm
-0.6V/ 30pA
(f)
Height (pm)
x (nm)
(g)
5nm
-0.6V/ 0.1pA
(h)
(i)
100nm
-1V/ 30pA
(j)
10nm
-0.5V/100pA
Height (pm)
x (nm)
(k)
5nm
-0.5V/100pA
(l)

**Fig. S2**: STM topography of (a-h) $Sm_{0.8}Eu_{0.2}B_6$ and (i-l) $Sm_{0.7}Ce_{0.3}B_6$. (a) Large-scale STM topography of the cleaved $Sm_{0.8}Eu_{0.2}B_6$ sample. (b) The atomically resolved structure of a typical *disordered* 1×2 (2×1) reconstructed surface and a featured line-profile of Z-height. (c) The Fourier transform of (b), showing unreconstructed Bragg peaks (1×1, white circles) and 1×2 (2×1) reconstructions (blue circle). (d) A boundary between a uniformly non-reconstructed 1×1 surface and the reconstructed 1×2 (2×1) surface. (e) The zoom-in STM topography and (f) its height line-profile shows a 0.1 nm step at the boundary, suggesting that this particular 1×1 non-reconstructed surface has a boron termination. (g) The atomically-resolved B-terminated surface and (h) its Fourrier transform with a 1×1 Bragg peak circled in white. Ripple-like inhomogeneity with a subatomic peak-to-valley height variation of <~50 pm can be observed on a few-nanometer scale in (g), as is typical for alloys, and represents inhomogeneity in the Eu/Sm sublattice beneath the B termination layer (see analysis in Fig. S3). (i) A large-scale STM topography of the cleaved $Sm_{0.7}Ce_{0.3}B_6$ sample. (j) A highly disordered surface, with featured line-profile of Z-height. (k) Zooming in on the 1×2 (2×1) reconstructed surface reveals in-plane fluctuations on the length scale of ~1nm, slightly shorter than the typical length scale in $Sm_{0.8}Eu_{0.2}B_6$ (~1.5nm) as expected given the higher doping level. (l) The corresponding Fourier transform shows a complex surface reconstruction, including 1×2 (green circle) and faint $\sqrt{2}\times\sqrt{2}$ (red circle) features. No large non-reconstructed surface was found on the surface of cleaved $Sm_{0.7}Ce_{0.3}B_6$ in surveys over 4 separate 500x500 $nm^2$ regions.

**Figure S3**

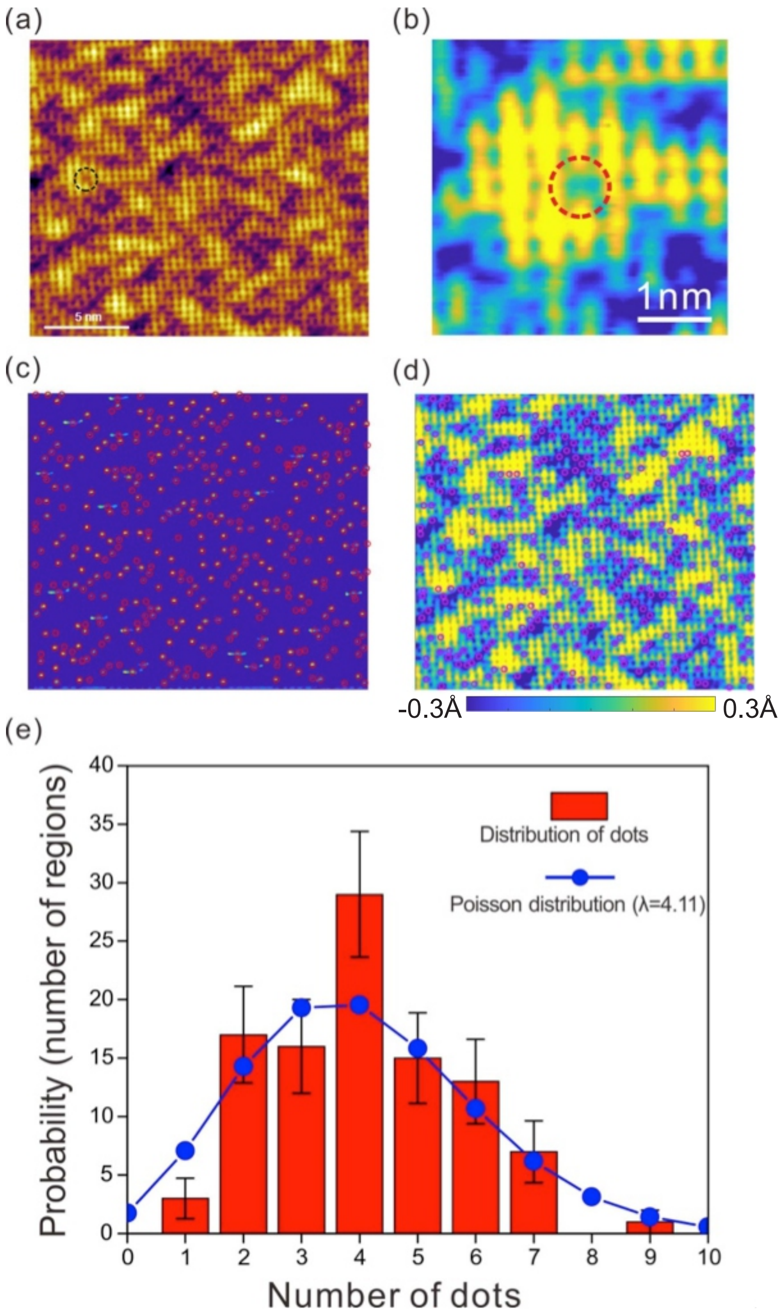


**Fig. S3**: Uniform alloying. (a) An interstitial single-site defect on the non-reconstructed B-termination of $Eu_{0.2}Sm_{0.8}B_6$ in Fig. S2(g) is circled, and is suggestive of a single-atom defect immediately beneath the boron termination layer. (b) A close-up to show a dim site with a yellow-hot color scale. A single-site (±2Å) window surrounding the defect is selected as a template. (c) Normalized cross-correlation between the selected template and the whole image reveals 411 similar sites (21% of sites), approximately matching the nominal 20% Eu doping. Circles indicate the center of mass of these peaks, and a close evaluation will reveal that horizontally-separated peaks are not always resolved. Manually correcting for

this and for ~5 apparent false positives results in a doping fraction of 22%. This estimate is consistent with the nominal doping value, given that statistical error bars are ±1.1% and systematic error likely rises to a similar or larger level. (d) The attributed Eu sites (correlation peak centroids) are overlaid on the STM image. (e) A histogram shows the distribution of attributed Eu densities, when the scanned surface is divided into 100 equal-sized regions. This distribution is compared with the Poisson distribution ($\lambda = 4.11 = 411/100$), revealing that the distribution of dopant Eu atoms is consistent with expectations for a fully random (non-clustered) configuration.

**Figure S4**

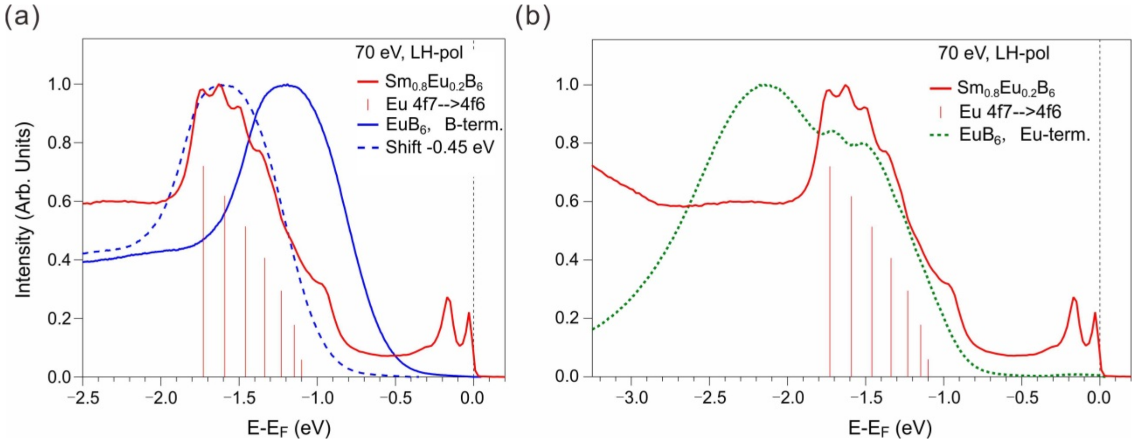


**Fig. S4**: 4*f* photoemission of $Sm_{0.8}Eu_{0.2}B_6$ and $EuB_6$. (a) Low energy features from the UV photoemission spectrum (PES) of $Sm_{0.8}Eu_{0.2}B_6$ is fitted with 4*f* multiplet ($4f^7$ to $4f^6$) numerical calculations [32], and compared with PES of pure $EuB_6$ with B-terminated cleaved surface (solid and dashed blue lines). (b) The low energy features from UV-PES of $Sm_{0.8}Eu_{0.2}B_6$ are compared with PES of pure $EuB_6$ with a Eu-terminated cleaved surface (dashed green line). The 4*f* photoemission of $Sm_{0.8}Eu_{0.2}B_6$ is incompatible with any significant admixture of pure $EuB_6$. The individual Eu multiplet peaks in $Sm_{0.8}Eu_{0.2}B_6$ are significantly narrower than in $EuB_6$, suggesting a very different local environment.

## Figure S5

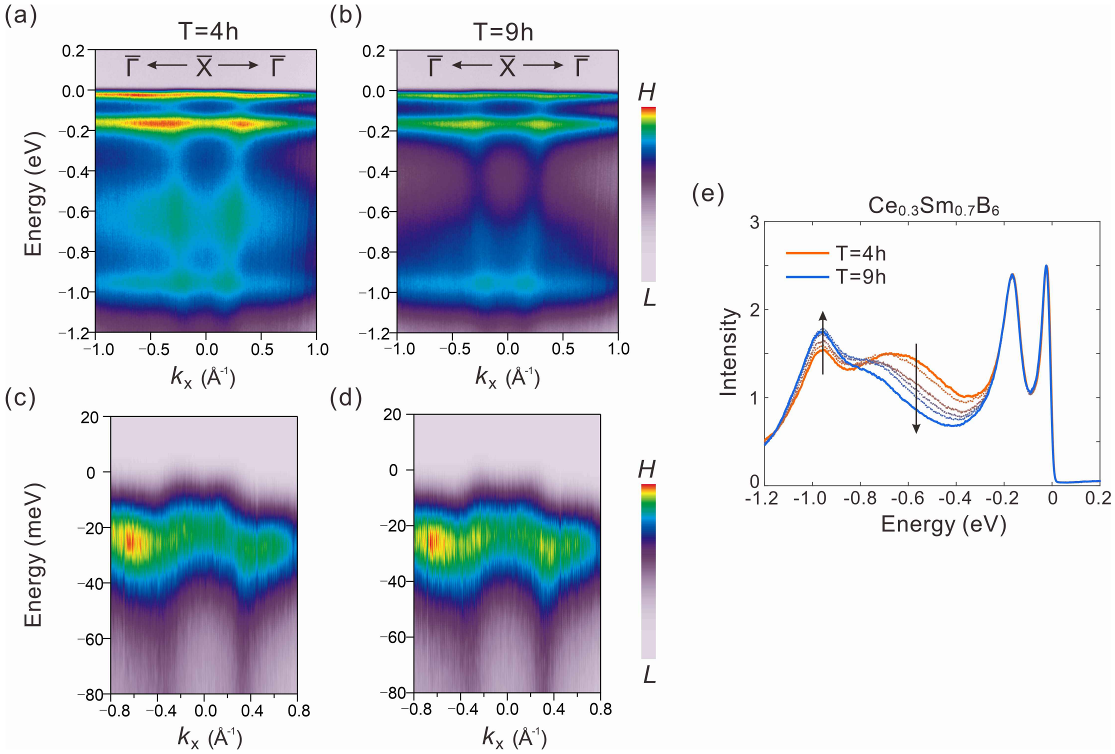


**Fig. S5.** Time-dependent photoemission spectra of $Sm_{0.7}Ce_{0.3}B_6$. (a-b) The same low-temperature ARPES measurement along $\overline{X}$ - $\overline{\Gamma}$ - $\overline{X}$ was performed (a) 4 hours and (b) 9 hours after sample cleavage. (c-d) A zoom-in near the Fermi level after (c) 4 hours (d) 9 hours, showing qualitatively identical spectra. The surface state Fermi momentum in each image is $k_F$~0.2Å$^{-1}$. No Fermi-level feature is present at the extrapolated Fermi momentum of the bulk 5*d* band ($k_F$~0.38Å$^{-1}$). (e) The momentum-integrated ARPES intensity as the function of time after cleavage, with constant intensity assigned to Kondo-associated features at the Fermi level. Dashed lines represent curves taken with interval of 1 hour between (orange) 4 hours and (blue) 9 hours after cleavage, and the arrows note the time progression.

**Figure S6**

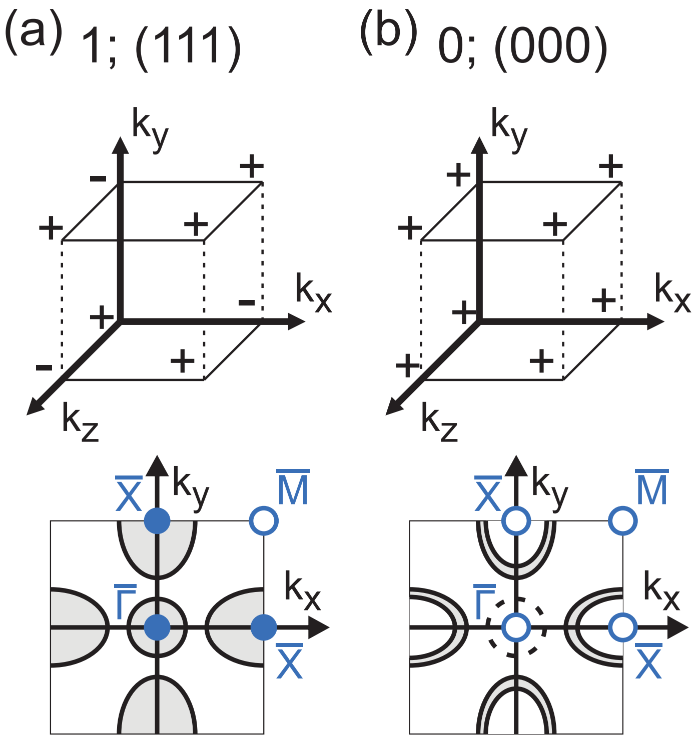


**Fig. S6.** Topological interpretation of $SmB_6$ band structure. (a) The strong TI topological invariants attributed to $SmB_6$ from DFT and bulk band structure measurements are shown above a diagram showing the bulk X-point symmetry inversions (following the convention in Ref. [18]). A compatible Fermi surface is shown at the bottom, with gray/white shading alternating across singly-degenerate Fermi contours. (b) A hypothetical non-TI scenario is shown. Though a non-TI bulk band structure has not been proposed to our knowledge, a topologically trivial interpretation of ARPES surface states that would be consistent with such a band structure is predicted in Ref. [20], matching the scenario at bottom.

**Figure S7**

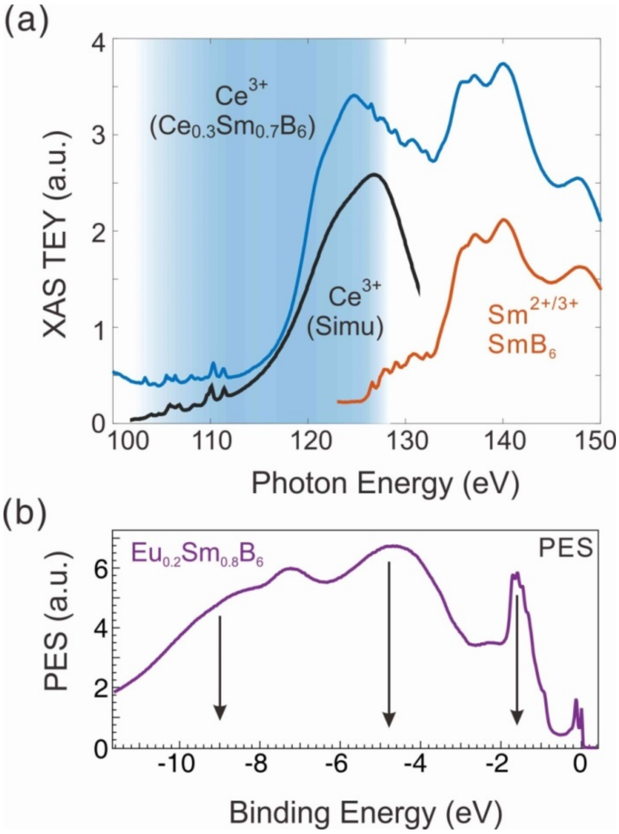


**Fig. S7.** Multiplet symmetries in $SmB_6$ alloys. (a) XAS measurements on $Ce_{0.3}Sm_{0.7}B_6$. The red curve is the data of pristine $SmB_6$ and the blue one is from $Ce_{0.3}Sm_{0.7}B_6$. The N-edge X-ray absorption spectrum of Ce is fitted with an atomic multiplet simulation for $Ce^{3+}$ (black line), and shaded with blue. (b) Angle-integrated photoemission measurements on $Eu_{0.2}Sm_{0.8}B_6$ obtained at photon energy hν=70eV.

**Figure S8**

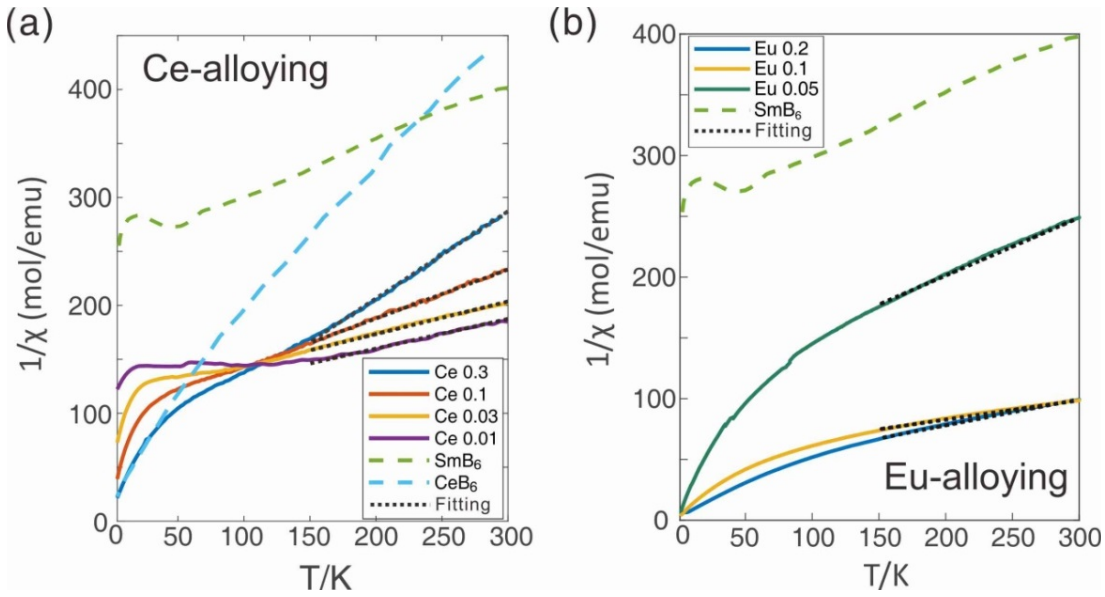


**Fig. S8.** The fitting of magnetic susceptibility. (a) The fitting of inverse susceptibility of Ce-alloyed $SmB_6$. (b) The fitting of inverse susceptibility of Eu-alloyed $SmB_6$.

**Figure S9**

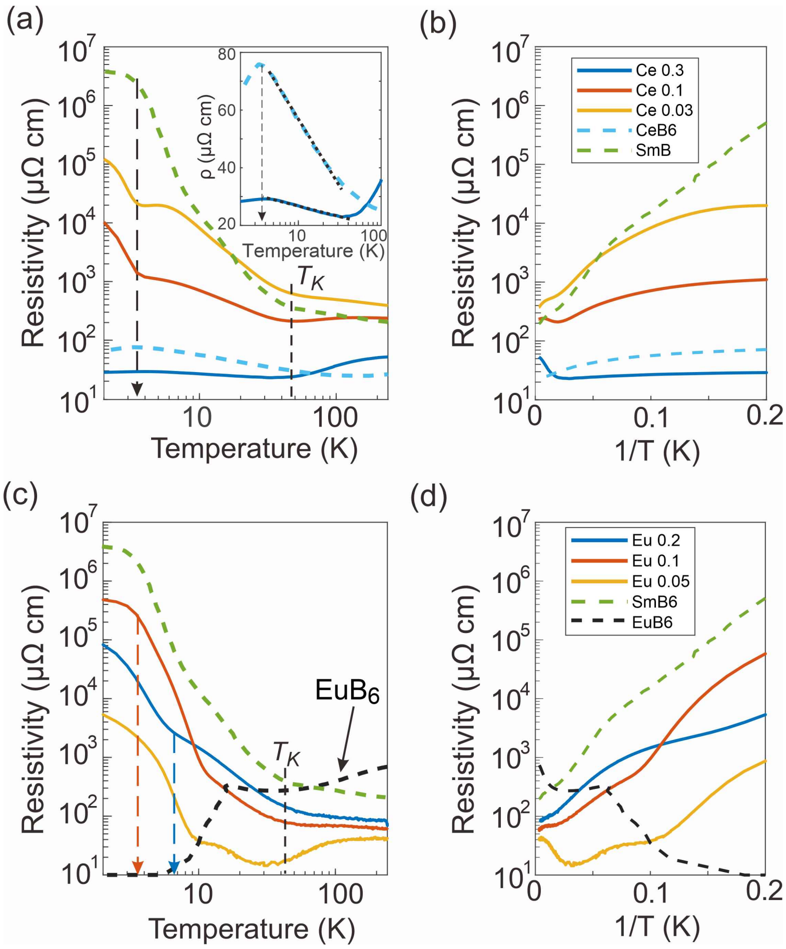


**Fig. S9.** The thermal activation behavior of resistivity in alloyed $SmB_6$. (a)-(b) The T-dependent bulk resistivity of (a) Ce-alloyed and (b) Eu-alloyed $SmB_6$, reproduced from Fig. 3(c-d) in the main text. (c-d) The resistivity of (c) Ce-alloyed and (b) Eu-alloyed $SmB_6$ is plotted on log(ρ)-(1/T) axes to show the thermal activation behavior.

**Figure S10**

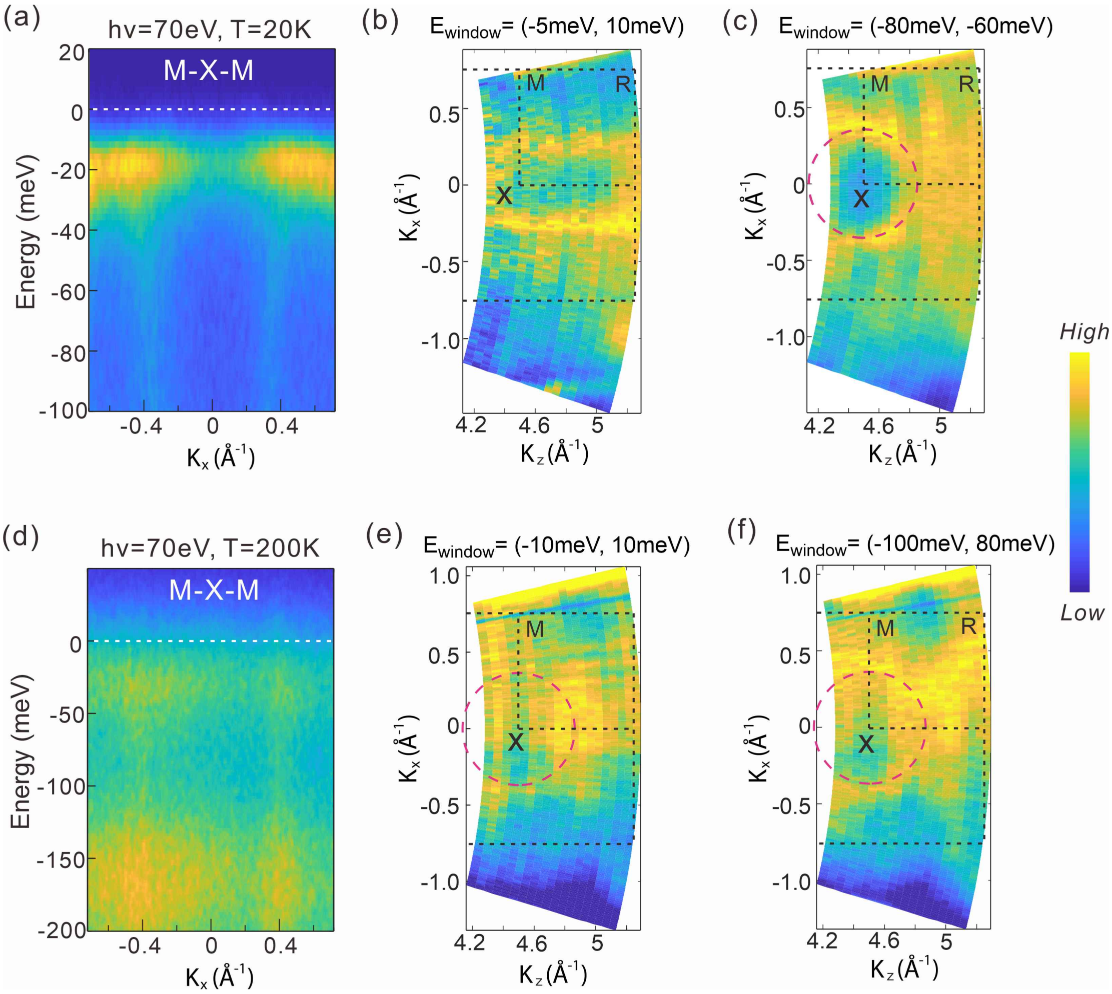


**Fig. S10.** Verification of two dimensional nature of the in-gap states in $Sm_{0.7}Ce_{0.3}B_6$ by incident photon energy dependence experiment. (a) An ARPES cut along the M-X-M direction with hv=70eV at T=20K. (b) The $k_x$-$k_z$ mapping of in-gap states, with intensity integrated from -5 meV to +10 meV from the Fermi level. (c) The $k_x$-$k_z$ mapping of the 5*d* bands beneath the Fermi level, with intensity integrated from -80meV to -60meV. The photon energy is varied from 62eV to 98eV with a step of 2eV, and used the measurement geometry of panel (a). The dispersive 5d band is overlaid with a dashed contour, as a guide to the eye. Because of the fixed geometry, the orthogonal ($k_y$) axis coordinate deviates from the $\overline{X}$ -point by -0.06Å$^{-1}$ to +0.14Å$^{-1}$ across the measured range, which will yield a small ~3.5% shift in the $k_x$ coordinate of the surface state at the far right of the graph, assuming an elliptical band contour. (d-f) The same measurements as (a-c) but with T=200K. Panel (f) is obtained at a slightly deeper binding energy than panel (c) to reduce background from the broader 4f bands.

**Figure S11**

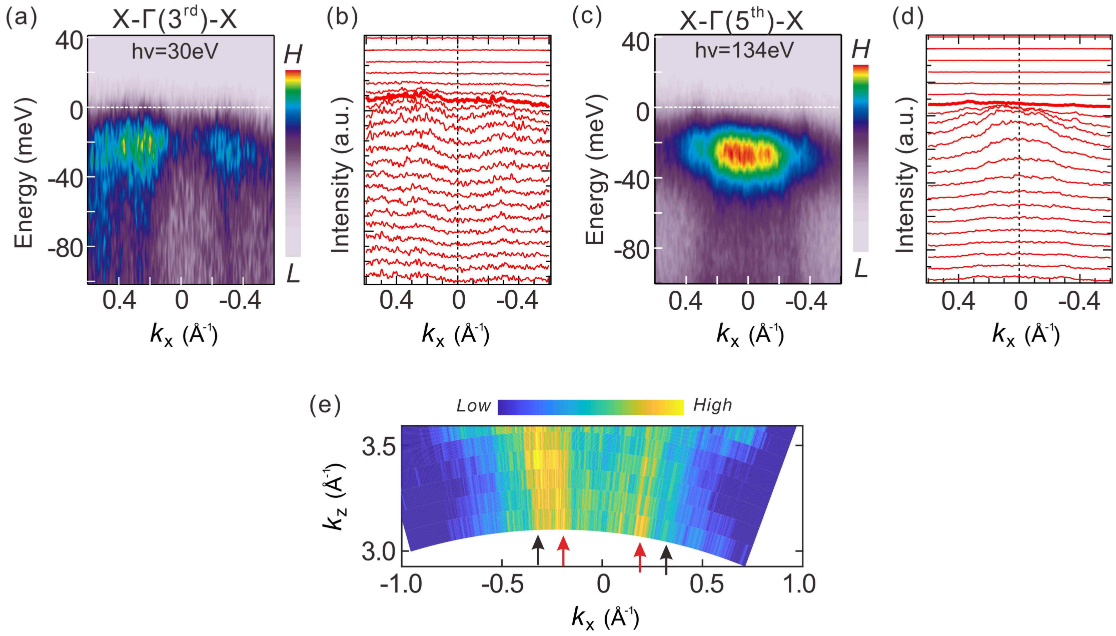


**Fig. S11.** The searching of possible surface states at the Γ point of $Sm_{0.9}Ce_{0.1}B_6$. (a) An ARPES cut over the X-Γ-X at hv=30eV which corresponds with the 3rd Γ point along the $k_z$ direction. (b) Momentum distribution curves for panel (a), with a 7 meV step size. (c) An ARPES cut along the X-Γ-X axis at hv=134eV which corresponds with the 5th Γ point along the $k_z$ direction. (d) Momentum distribution curves for panel (c), with a 7 meV step. The Fermi level in (b) and (d) is indicated with a thicker red line. (e) The $k_x$-$k_z$ Fermi level map, with incident photon energy varied from 30eV to 38eV. Arrows indicate $k_X$ momenta associated with (black) the surface state surrounding the $\overline{X}$ -point and (red) a candidate $\overline{\Gamma}$ -point surface state.

**Figure S12**

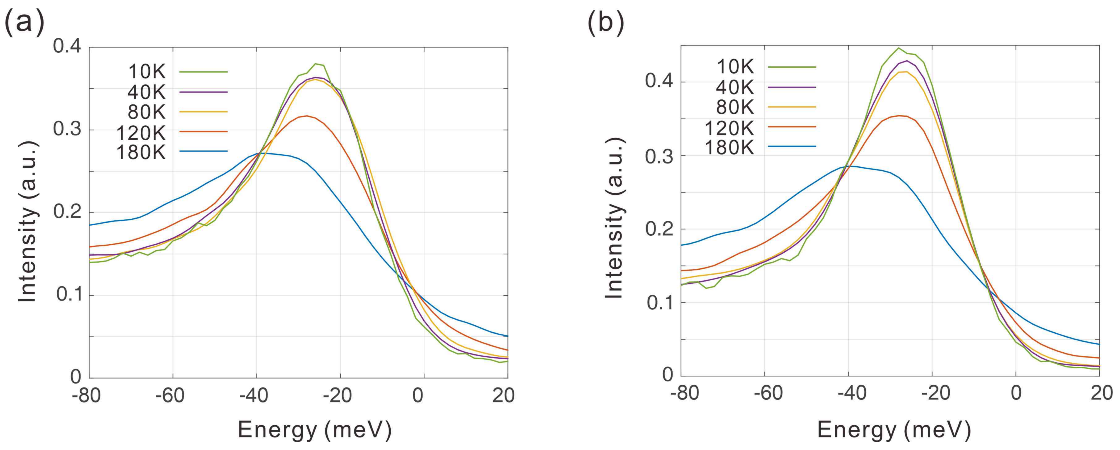


**Fig. S12.** The *f*-electron spectral contour versus temperature. (a) Energy dispersion curves at $k_y$=±1 Å$^{-1}$ from Fig. 2(b) in the main text. (b) Energy dispersion curves at $k_y$=±0.75Å$^{-1}$ (the high symmetry X-point) from the temperature-dependent spectra.

These curves are symmetrized across the $k_X$ axis, and integrated intensity is normalized.

**Reference:**


1. S. Yeo, K. Song, N. Hur, Z. Fisk, P. Schlottmann, Effects of Eu doping on $SmB_6$ single crystals, *Phys. Rev. B* **85**, 115125 (2012).
2. J. M. Lawrence, et al. Kondo hole behavior in $Ce_{0.97}La_{0.03}Pd_3$ *Phys. Rev. B* **53**, 12559 (1996)
3. M. H. Hamidian, et al. How Kondo-holes create intense nanoscale heavy-fermion hybridization disorder, *Proc. Natl. Acad. Sci. USA,* **108**, 18233-18237 (2001).
4. P. F. S. Rosa, A. Oostra, J. D. Thompson, P. G. Pagliuso, Z. Fisk, Unusual Kondo-hole effect and crystal-field frustration in Nd-doped $CeRhIn_5$, *Phys. Rev. B* **94**, 045101 (2016) .
5. J. D. Thompson, Holes in a Kondo lattice, *Proc. Natl. Acad. Sci. USA* **108**, 18191 (2011).
6. R. Sollie, P. Schlottmann, A simple theory of the Kondo hole. *J. Appl. Phys*. **96**, 5478–5480 (1991).
7. B. Skinner, Properties of the donor impurity band in mixed valence insulators, *Phys. Rev. Mater.* **3**, 104601 (2019).
8. Y. S. Eo et al. Transport gap in $SmB_6$ protected against disorder, *Proc. Natl. Acad. Sci. USA*, **116**, 12638-12641 (2019).
9. H. He, et al. Irreversible proliferation of magnetic moments at cleaved surfaces of the topological Kondo insulator $SmB_6$, *Phys. Rev. B* **95**, 195126 (2017).
10. P. Lutz et al. Valence characterisation of the subsurface region in $SmB_6$, *Philos. Mag.* **96**, 3307 (2016).
11. J.D. Denlinger, et al. $SmB_6$ Photoemission: Past and Present, *JPS Conf. Proc.* **3**, 017038 (2014).
12. S. Suga, et al. Spin-Polarized Angle-Resolved Photoelectron Spectroscopy of the So-Predicted Kondo Topological Insulator $SmB_6$. *J. Phys. Soc. Jpn.* **83**, 014705 (2014).
13. N. Xu, et al. Direct observation of the spin texture in SmB6 as evidence of the topological Kondo insulator, *Nat. Commun.* **5**, 4566. (2014).
14. N. Xu, H. Ding, and M. Shi, Spin- and angle-resolved photoemission on the topological Kondo insulator candidate: $SmB_6$, *J. Phys. Cond. Matter*, **28**, 36 (2016).
15. Y. Ohtsubo, et al, Non-trivial surface states of samarium hexaboride at the (111) surface, *Nat. Commun*. **10**, 2298 (2019).
16. E. Frantzeskakis, et al. Kondo Hybridization and the Origin of Metallic States at the (001) Surface of $SmB_6$, *Phys. Rev. X* **3**, 041024 (2013).
17. M. Dzero, K. Sun, V. Galitski, P. Coleman, Topological Kondo Insulators, *Phys. Rev. Lett.* **104**, 106408 (2001).
18. L. Fu, C. L. Kane, and E. J. Mele, Topological Insulators in Three Dimensions, *Phys. Rev. Lett*. **98**, 106803 (2007).
19. F. Siek, et al. Angular momentum–induced delays in solid-state photoemission enhanced by intra-atomic interactions, *Science* **357**, 1274 (2017).
20. P. Hlawenka, et al. Samarium hexaboride is a trivial surface conductor, *Nat.*

*Commun.* **9**, 517 (2018).
21. S. Rößler, et al. Hybridization gap and Fano resonance in $SmB_6$, *Proc. Nat. Acad. Sci.*, **111**, 4798 (2014).
22. C. E. Matt et al. Consistency between ARPES and STM measurements on $SmB_6$, *Phys. Rev. B* **101**, 085142 (2020).
23. H. He, et al. Irreversible proliferation of magnetic moments at cleaved surfaces of the topological Kondo insulator $SmB_6$, *Phys. Rev. B* **95**, 195126 (2017).
24. Y. Takakuwa, S. Suzuki, T. Sagawa, Photoemission Measurements of $EuB_6$, *Jpn. J. Appl. Suppl.* **17**, 284 (1978).
25. J. A. Colon-Santana, et al. Effect of gadolinium doping on the electronic band structure of europium oxide *Phys. Rev. B* **85**, 014406 (2012).
26. Hartree-Fock Slater Condon parameters were obtained from the Cowan code (see https://www.tcd.ie/Physics/people/Cormac.McGuinness/Cowan/)
27. E. Anderson, et al. LAPACK User's Guide, 3rd ed. (SIAM, Philadelphia, 1999).
28. A. Maurya, R. Kulkarni, A. Thamizhavel, D. Paudyal, S.K. Dhar Kondo lattice and antiferromagnetic behavior in quaternary $CeTAl_4Si_2$ (T = Rh, Ir) single crystals, *J. Phys. Soc. Jpn.* **85**, 034720 (2016).
29. Y. Singh, R.S. Sannabhadti, S. Ramakrishnan, Low-temperature properties of a new Kondo Lattice compound $Yb_2Ir_3Sn_5$, arXiv:cond-mat/0510583
30. C. Terzioglu, D.A. Browne, R.G. Goodrich, A. Hassa, Z. Fisk, EPR and magnetic susceptibility measurements on $CeB_6$, *Phys. Rev. B* **63**, 235110 (2001).
31. J. D. Denlinger, J. W. Allen, J.-S. Kang, K. Sun, J.-W. Kim, J. H. Shim, B. I. Min, D.-J. Kim, and Z. Fisk, Temperature Dependence of Linked Gap and Surface State Evolution in the Mixed Valent Topological Insulator $SmB_6$, arXiv:1312.6637 (2014).
32. F. Gerken, Calculated photoemission spectra of the 4f states in the rare-earth metals, *J. Phys. F: Met. Phys.* 13, 703 (1983)
33. X.-L. Qi and S.-C. Zhang, Topological insulators and superconductors, Colloquium: Topological insulators, *Rev. Mod. Phys.* **83**, 1057 (2011).
34. M. Z. Hasan and C. L. Kane, Topological insulators, *Rev. Mod. Phys.* **82**, 3045 (2010).
35. M. Liu et al. Crossover between Weak Antilocalization and Weak Localization in a Magnetically Doped Topological Insulator, *Phys. Rev. Lett.* **108**, 036805 (2012)
36. Y. Xu et al. Disorder enabled band structure engineering of a topological insulator surface, *Nat. Commun.* **8**. 14081 (2017).
